# Supplementary material for: ReDraft, Don't Just Distill: Reference-Driven Revision for Continual VLLM Post-Training
Source: arXiv:2609.16639 source file (2026-09-22)
Supplement: Supplementary file 1 [file demo_box_styles.tex]

% Shared rounded-box styles for qualitative demos.
% Requires: \usepackage[most]{tcolorbox}, float, placeins.

\makeatletter
\ifdefined\XeTeXrevision
  \@ifpackageloaded{fontspec}{}{\usepackage{fontspec}}
  \IfFontExistsTF{Latin Modern Mono}{%
    \newfontfamily\DemoMono{Latin Modern Mono}[Scale=MatchLowercase]%
  }{%
    \IfFontExistsTF{Menlo}{%
      \newfontfamily\DemoMono{Menlo}[Scale=MatchLowercase]%
    }{%
      \newcommand{\DemoMono}{\ttfamily}%
    }%
  }%
\else
  \ifdefined\luatexversion
    \@ifpackageloaded{fontspec}{}{\usepackage{fontspec}}
    \IfFontExistsTF{Latin Modern Mono}{%
      \newfontfamily\DemoMono{Latin Modern Mono}[Scale=MatchLowercase]%
    }{%
      \newcommand{\DemoMono}{\ttfamily}%
    }%
  \else
    \newcommand{\DemoMono}{\ttfamily}%
  \fi
\fi
\makeatother

\definecolor{DemoInputFrame}{HTML}{667085}
\definecolor{DemoInputTitle}{HTML}{475467}
\definecolor{DemoInputBack}{HTML}{F8FAFC}
\definecolor{DemoExampleFrame}{HTML}{4B5563}
\definecolor{DemoExampleTitle}{HTML}{374151}
\definecolor{DemoExampleBack}{HTML}{FFFFFF}
\definecolor{DemoWrongFrame}{HTML}{B95A45}
\definecolor{DemoWrongTitle}{HTML}{8E3B2A}
\definecolor{DemoWrongBack}{HTML}{FBF3F0}
\definecolor{DemoRightFrame}{HTML}{4A8F73}
\definecolor{DemoRightTitle}{HTML}{2F6B54}
\definecolor{DemoRightBack}{HTML}{F1F7F3}
\definecolor{DemoTemplateFrame}{HTML}{A07A33}
\definecolor{DemoTemplateTitle}{HTML}{7A5A1E}
\definecolor{DemoTemplateBack}{HTML}{FAF6EC}


\tcbset{
  demobase/.style={
    enhanced,
    breakable,
    boxrule=0.8pt,
    arc=2mm,
    left=7pt,
    right=7pt,
    top=6pt,
    bottom=6pt,
    toptitle=3pt,
    bottomtitle=3pt,
    lefttitle=7pt,
    righttitle=7pt,
    before skip=8pt,
    after skip=8pt,
    fontupper={\footnotesize\DemoMono\raggedright},
    fonttitle=\bfseries\small,
    coltitle=white,
  },
  demoinput/.style={
    demobase,
    unbreakable,
    fontupper={\normalfont},
    colback=DemoInputBack,
    colframe=DemoInputFrame,
    colbacktitle=DemoInputTitle,
    title={#1},
  },
  demoexample/.style={
    demobase,
    fontupper={\small\raggedright},
    colback=DemoExampleBack,
    colframe=DemoExampleFrame,
    colbacktitle=DemoExampleTitle,
    title={#1},
  },
  demowrong/.style={
    demobase,
    colback=DemoWrongBack,
    colframe=DemoWrongFrame,
    colbacktitle=DemoWrongTitle,
    title={Incorrect Rollout},
  },
  demoright/.style={
    demobase,
    colback=DemoRightBack,
    colframe=DemoRightFrame,
    colbacktitle=DemoRightTitle,
    title={Revised Response},
  },
  demotemplate/.style={
    demobase,
    colback=DemoTemplateBack,
    colframe=DemoTemplateFrame,
    colbacktitle=DemoTemplateTitle,
    title={#1},
  },
}
